# Supplementary material for: Atomistic origin of metal versus charge-density-wave phase separation in indium atomic wires on Si(111)
Source: arXiv:2106.03380 source file (2021-06-07)
Supplement: Supplementary file 1 [file Supp_material_for_Atomistic_origin_of_metal_CDW_phase_separation.pdf]

# Supplemental Material for:Atomistic origin of metal/charge-density-wave phase separation

Sun Kyu Song[1] and Han Woong Yeom[1,2]

[1]*Center for Artificial Low Dimensional Electronic Systems, Institute for Basic Science (IBS), Pohang 37673, Republic of Korea*

[2]*Department of Physics, Pohang University of Science and Technology (POSTECH), Pohang 37673, Republic of Korea*

| | Strong PFD ('M') | Weak PFD ('A') | Adatom cluster | Vacancy |
|---|---|---|---|---|
| # of defects | 433 | 110 | 46 | 41 |
| # of defects at domain boundaries | 272 | 39 | 15 | 21 |

TABLE S1. The number of the two PFDs, adatom clusters and vacancies counted in five STM images with the scanning area of 50 nm $\times$ 50 nm.

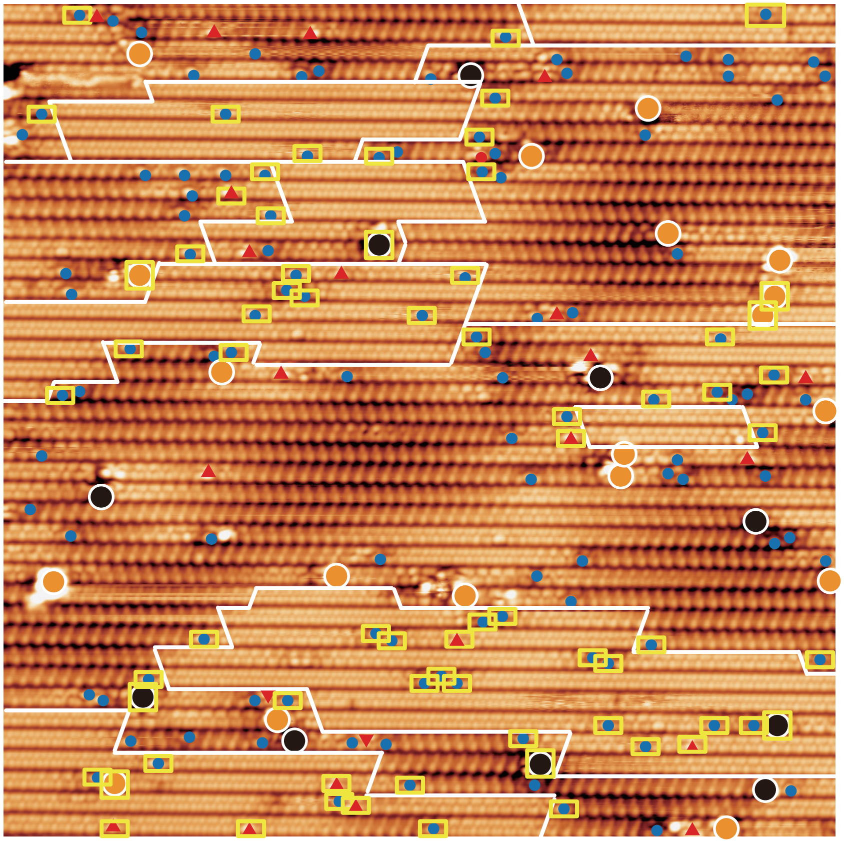

FIG. S1. STM image showing the phase boundaries between the metallic $4 \times 1$ phases and the insulating $8 \times 2$ phases. The blue dots and red triangles indicate the strong PFD ('M' shape) and the weak PFD ('A' shape), respectively. Orange circles and black circles indicate adatom clusters and vacancies, respectively. The defects located at the domain boundaries are marked with the yellow box.

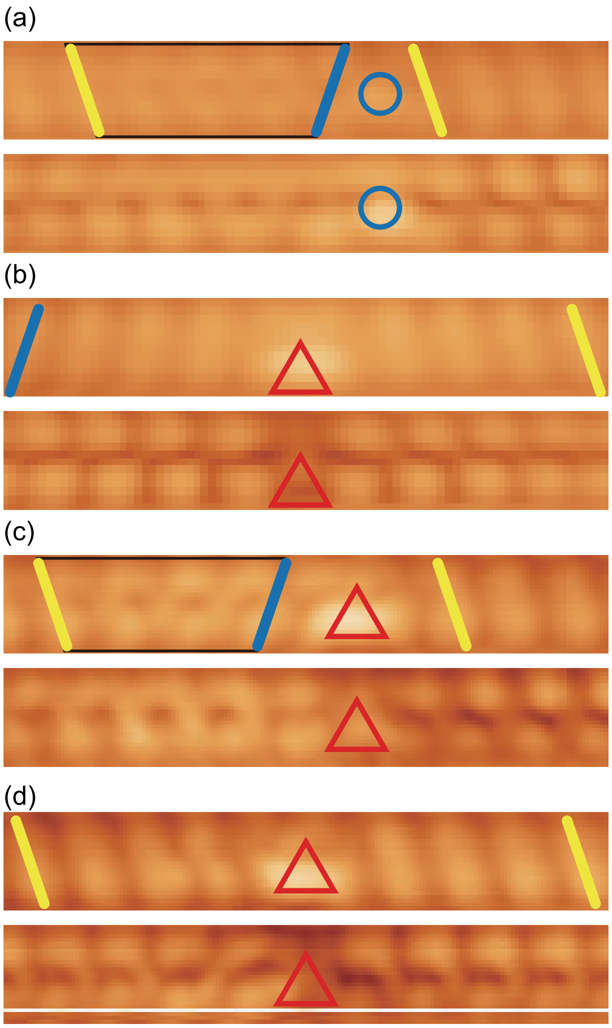


FIG. S2. Close-up STM images of the PFDs between two CDW domains. Blue circles and red triangles indicate the strong PFDs ('M' shape) and weak PFDs ('A' shape), respectively. Yellow and blue line indicate the oppsite CDW orientations. Black boxes indicate the topological solitons.

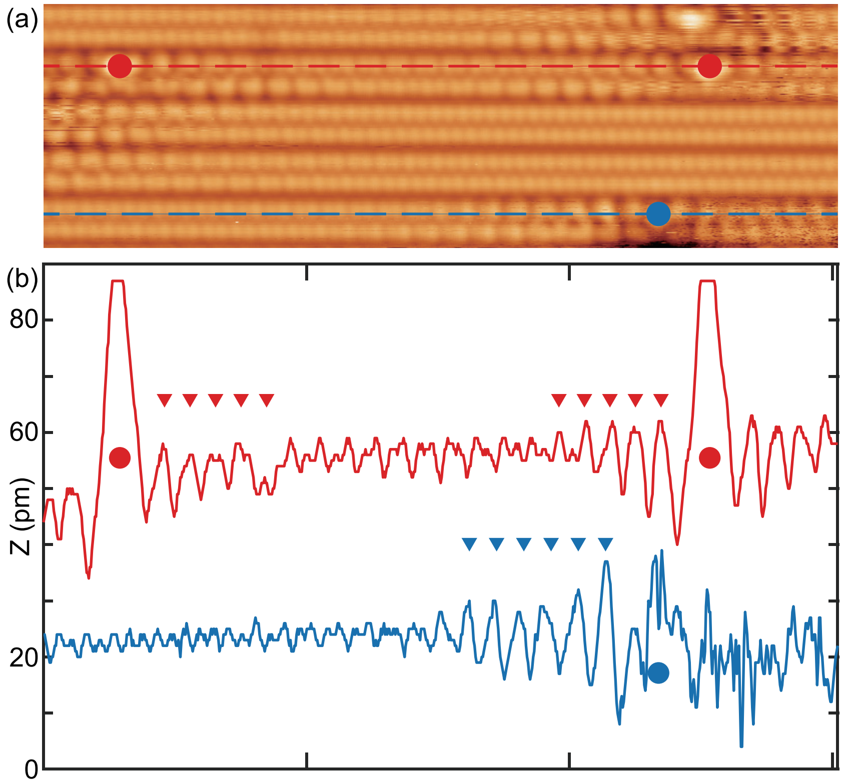


FIG. S3. (a) STM image ($V_S = -0.2$ V and $I_t = 100$ pA) showing the local lattice distortions induced by the PFDs taken at 140 K. (b) Height profiles corresponding to the dotted lines in (a). Circles indicate the position of the PFDs and the triangles indicate the $\times 2$ local lattice distortions.

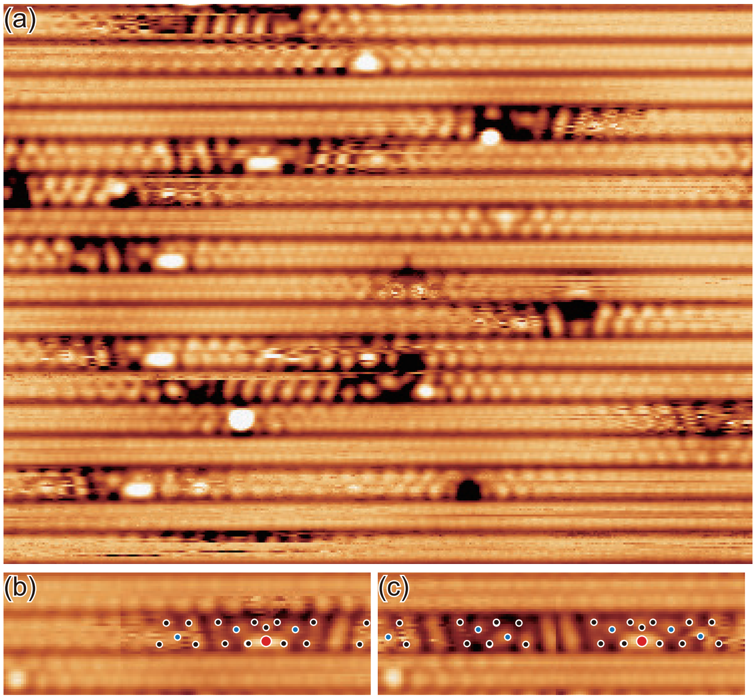


FIG. S4. (a) STM image ($V_S = -0.5$ V and $I_t = 100$ pA) showing the rapid motion of the strong PFDs taken at 120 K. The noisy stripes and the unclear structures of the strong PFDs indicate the mobility of the strong PFDs. (b) The appearance of the strong PFDs during STM measurements indicates the mobility of the strong PFDs.

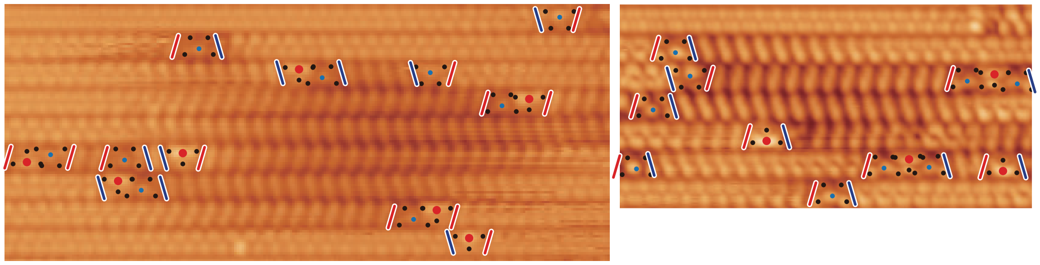

FIG. S5. STM topographic images ($V_s = -0.5$ V) of two small domains in $8 \times 2$ CDW state surrounded by PFDs and metallic domains at 95 K, without a single vacancy defect.
